# Supplementary material for: Towards Verifying Exact Conditions for Implementations of Density Functional Approximations
Source: arXiv:2408.05316 source file (2025-03-14)
Supplement: Supplementary file 1 [file supplemental.tex]

\section{Supplemental}
\label{sec:Supplemental}

\begin{figure}
    \centering
    \includegraphics[width=0.49\textwidth]{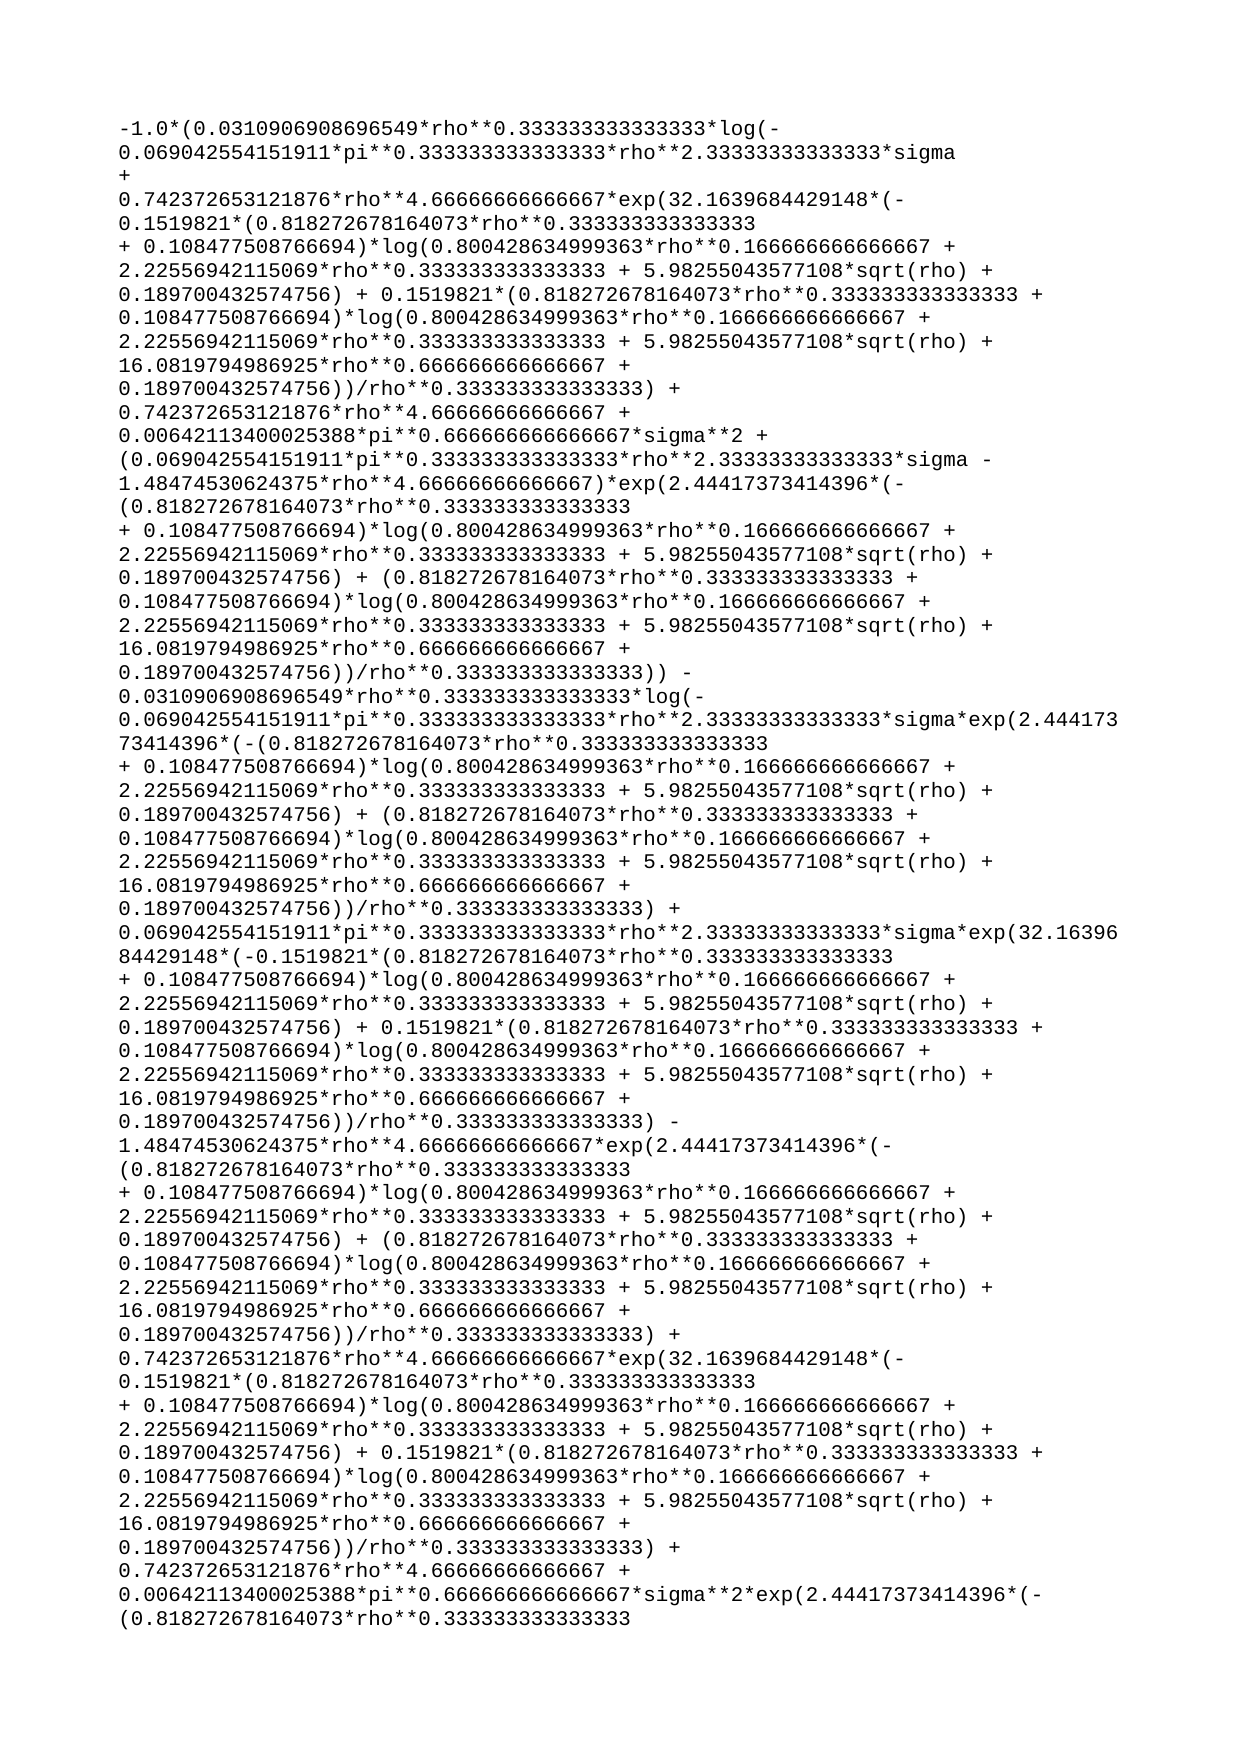}
    \caption{PBE Correlation Energy}
    \label{fig:pbe_correlation}
\end{figure}

\begin{figure}
    \centering
    \includegraphics[width=0.49\textwidth]{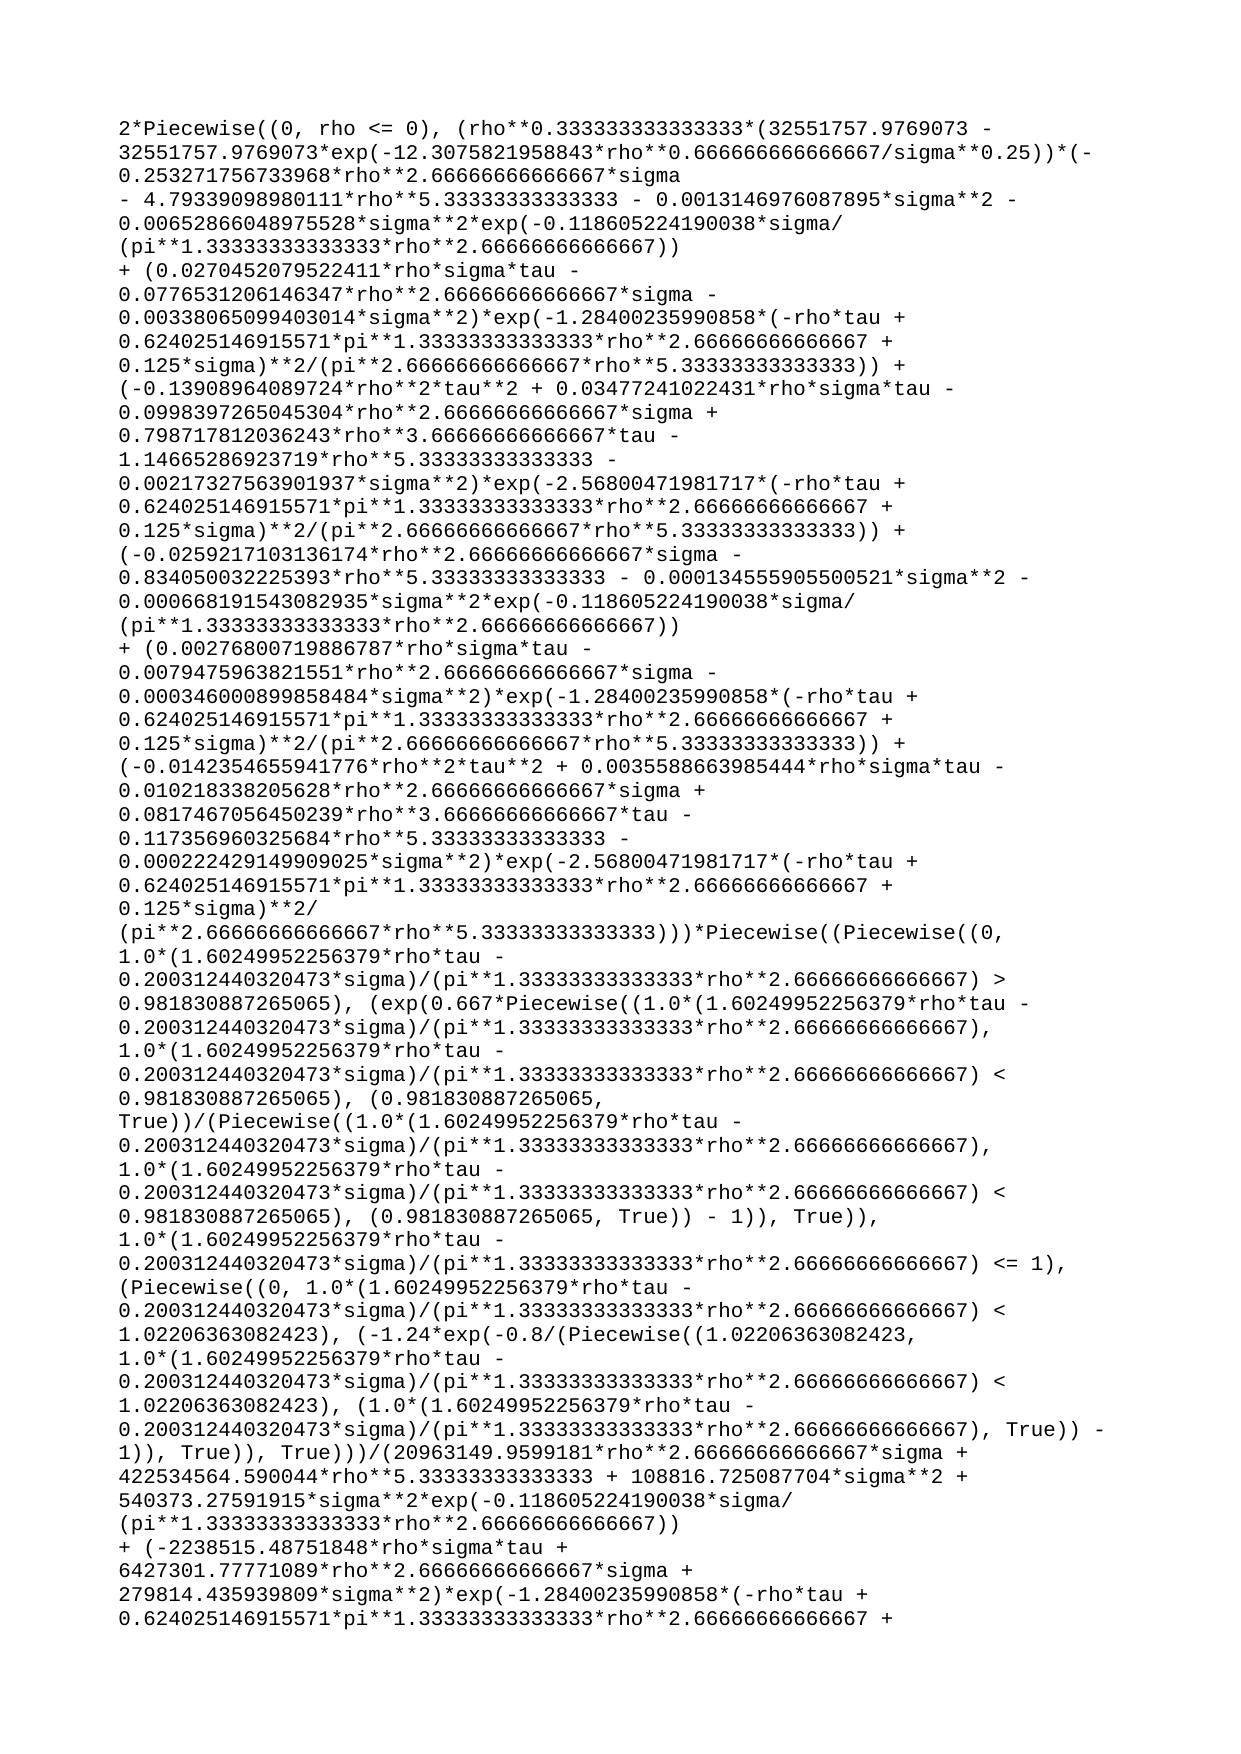}
    \caption{SCAN Exchange Energy}
    \label{fig:scan_exchange}
\end{figure}

\begin{figure}
    \centering
    \includegraphics[width=0.49\textwidth]{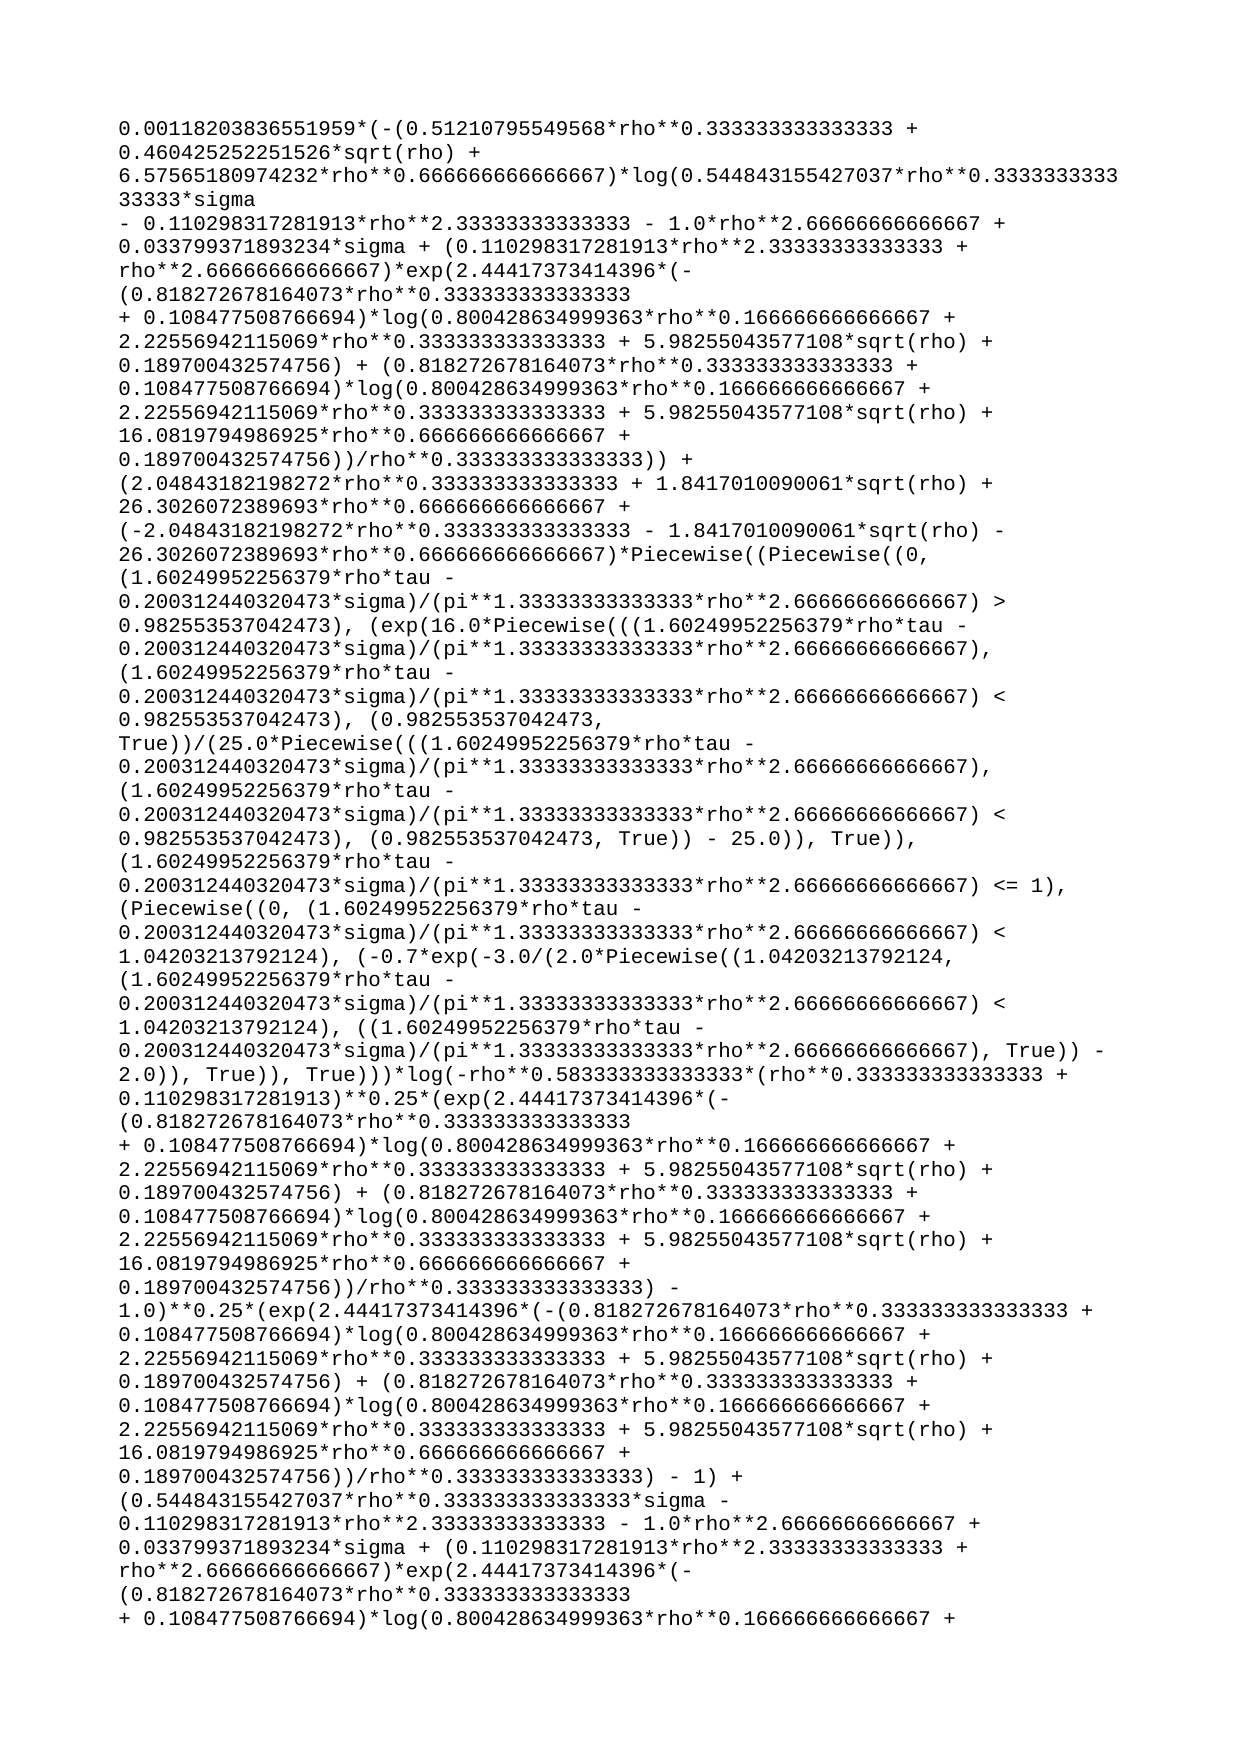}
    \caption{SCAN Correlation Energy}
    \label{fig:scan_correlation}
\end{figure}
